# Supplementary material for: Beyond Current Boundaries: Integrating Deep Learning and AlphaFold for Enhanced Protein Structure Prediction from Low-Resolution Cryo-EM Maps
Source: arXiv:2410.23321 source file (2024-10-30)
Supplement: Supplementary file 1 [file appendix.tex]

\appendix
\raggedbottom\sloppy

% ========== Appendix A
\clearpage
\section{Visualizations and Full Test Data}
 
\begin{figure}[!h]
    \centering
    \begin{subfigure}[t]{0.98\textwidth}
        \centering
        \includegraphics[width=\linewidth]{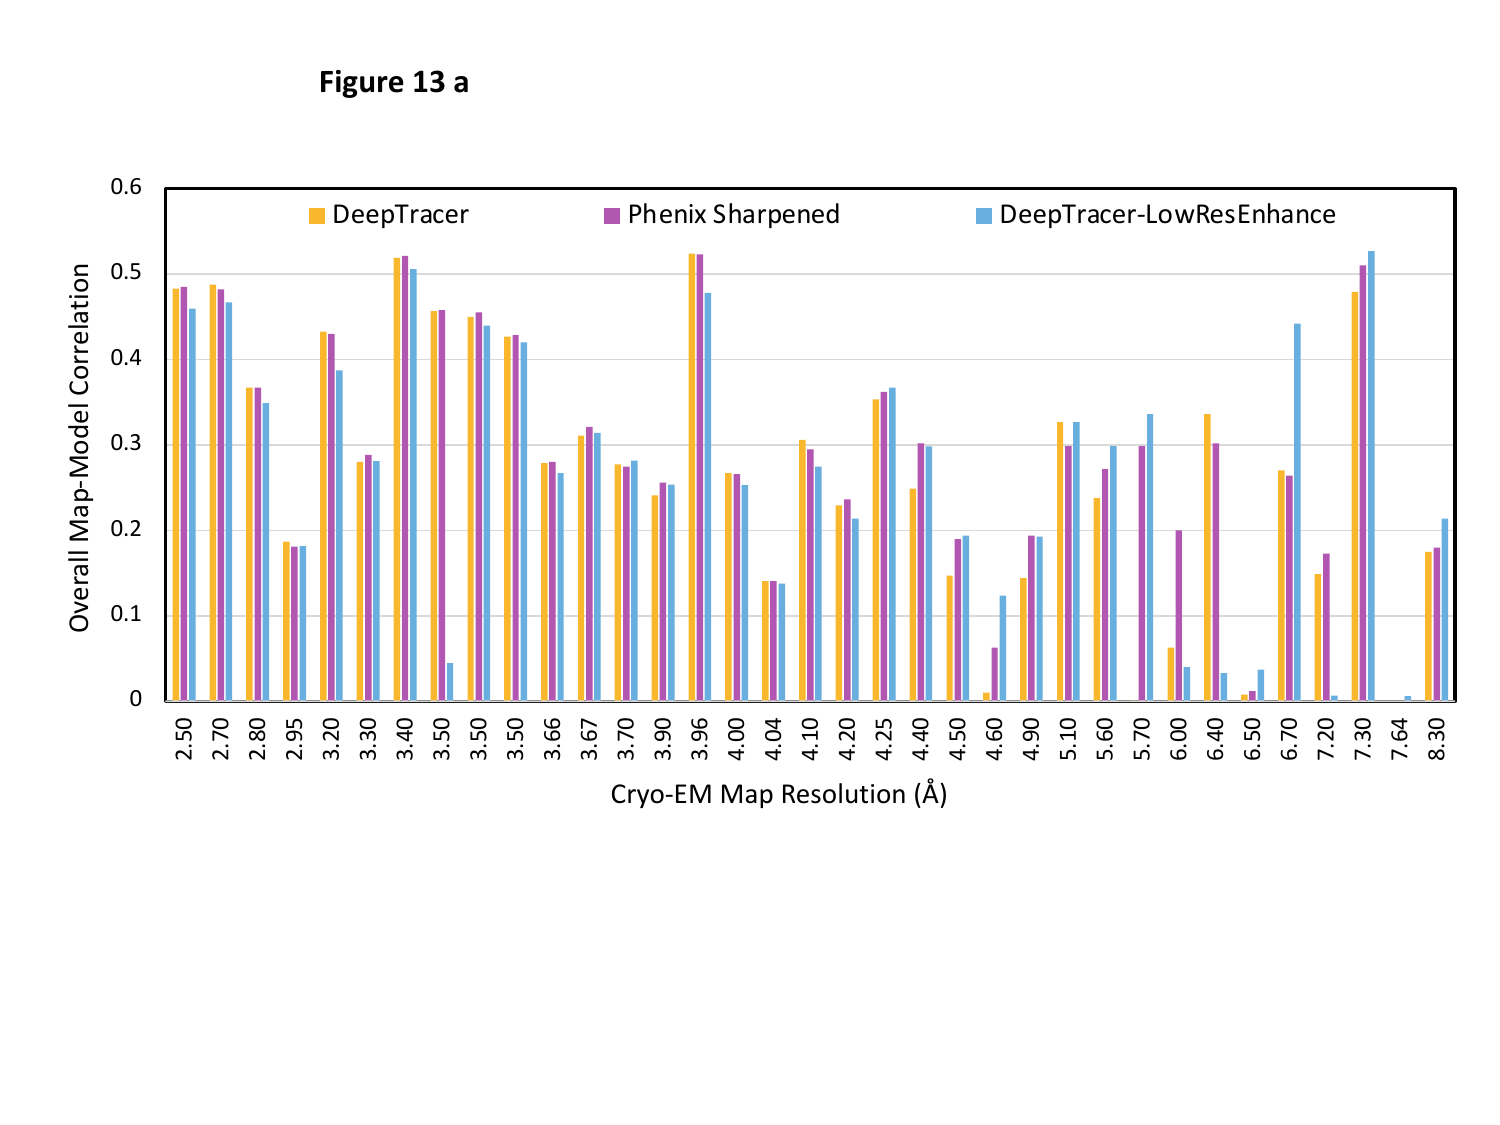}
        \caption{Overall map-model correlation comparison with resolution.}
    \label{fig:appendix-map-model-correlation_a}
    \end{subfigure}%

    \vspace{0.5cm} % Add some vertical space between the subfigures
    
    \begin{subfigure}[t]{0.98\textwidth}
        \centering
        \includegraphics[width=\linewidth]{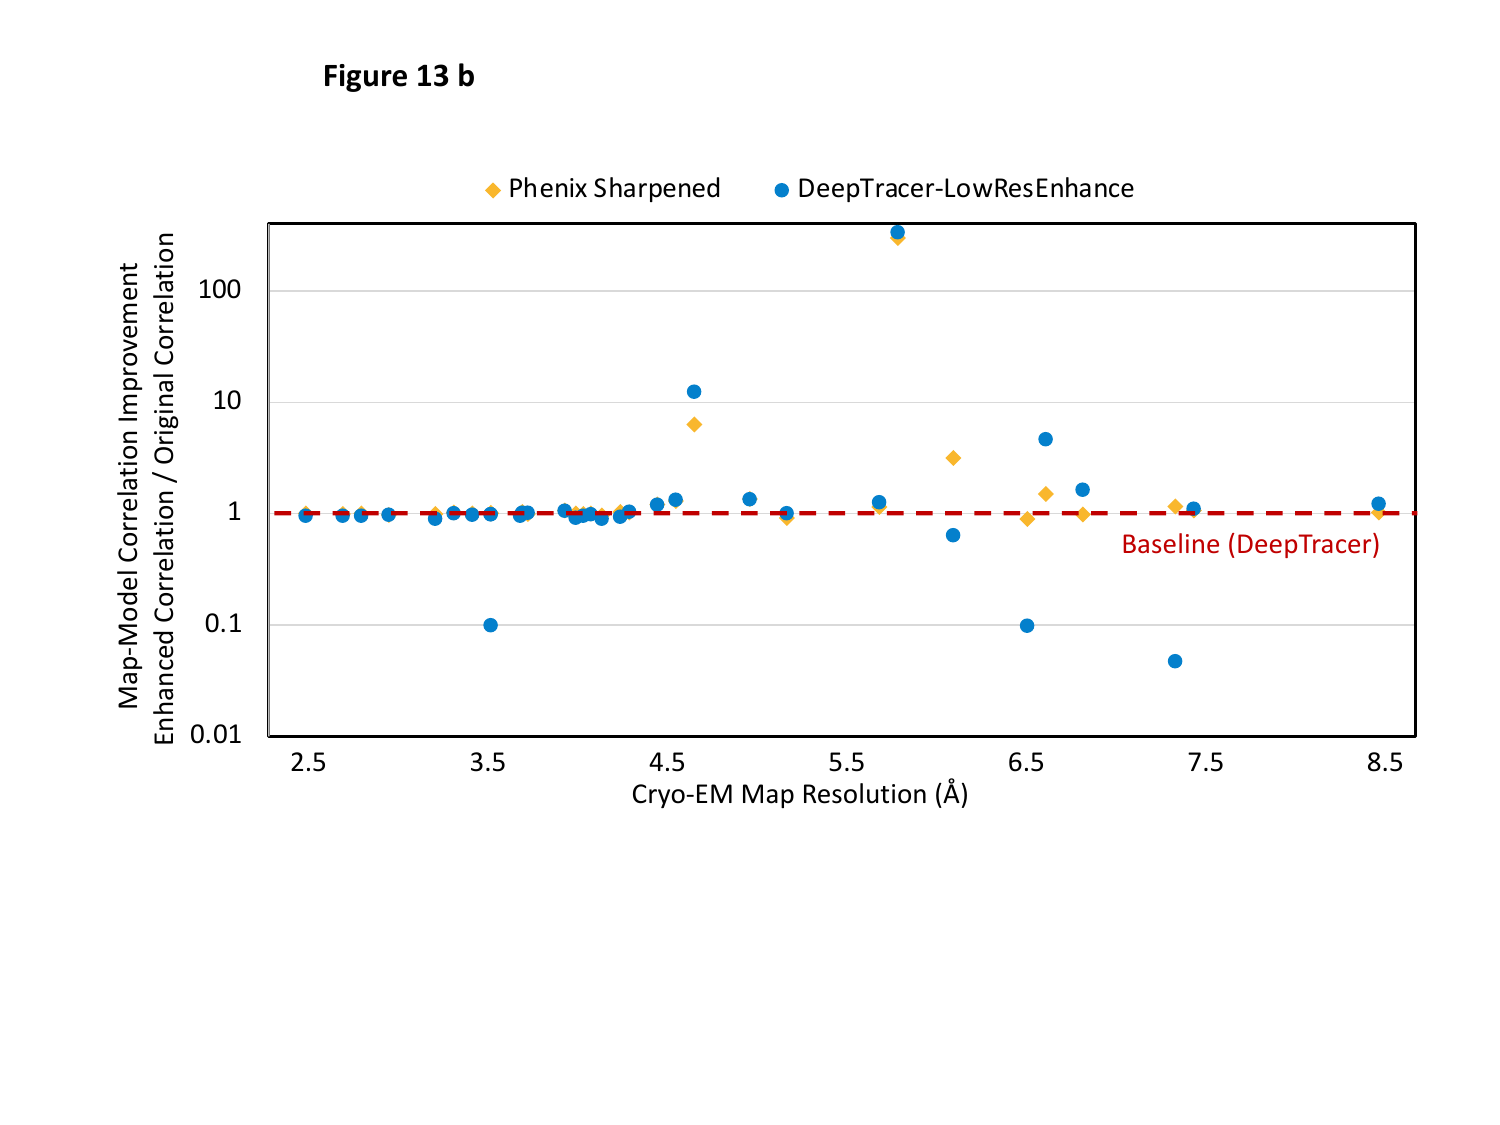}
    \caption{Overall map-model correlation of comparison models with DeepTracer baseline model.}
    \label{fig:appendix-map-model-correlation_b}
    \end{subfigure}
    \caption{Overall Map-Model Correlation Comparison between our proposed DeepTracer-LowResEnhance workflow, DeepTracer with Phenix sharpened maps, and original DeepTracer.}
    \label{fig:appendix-map-model-correlation}
\end{figure}

% You can reference the figure in your text by using \ref{fig:appendix-map-model-correlation}

\begin{figure}[!h]
    \centering
    \begin{subfigure}[t]{0.98\textwidth}
        \centering
        \includegraphics[width=\linewidth]{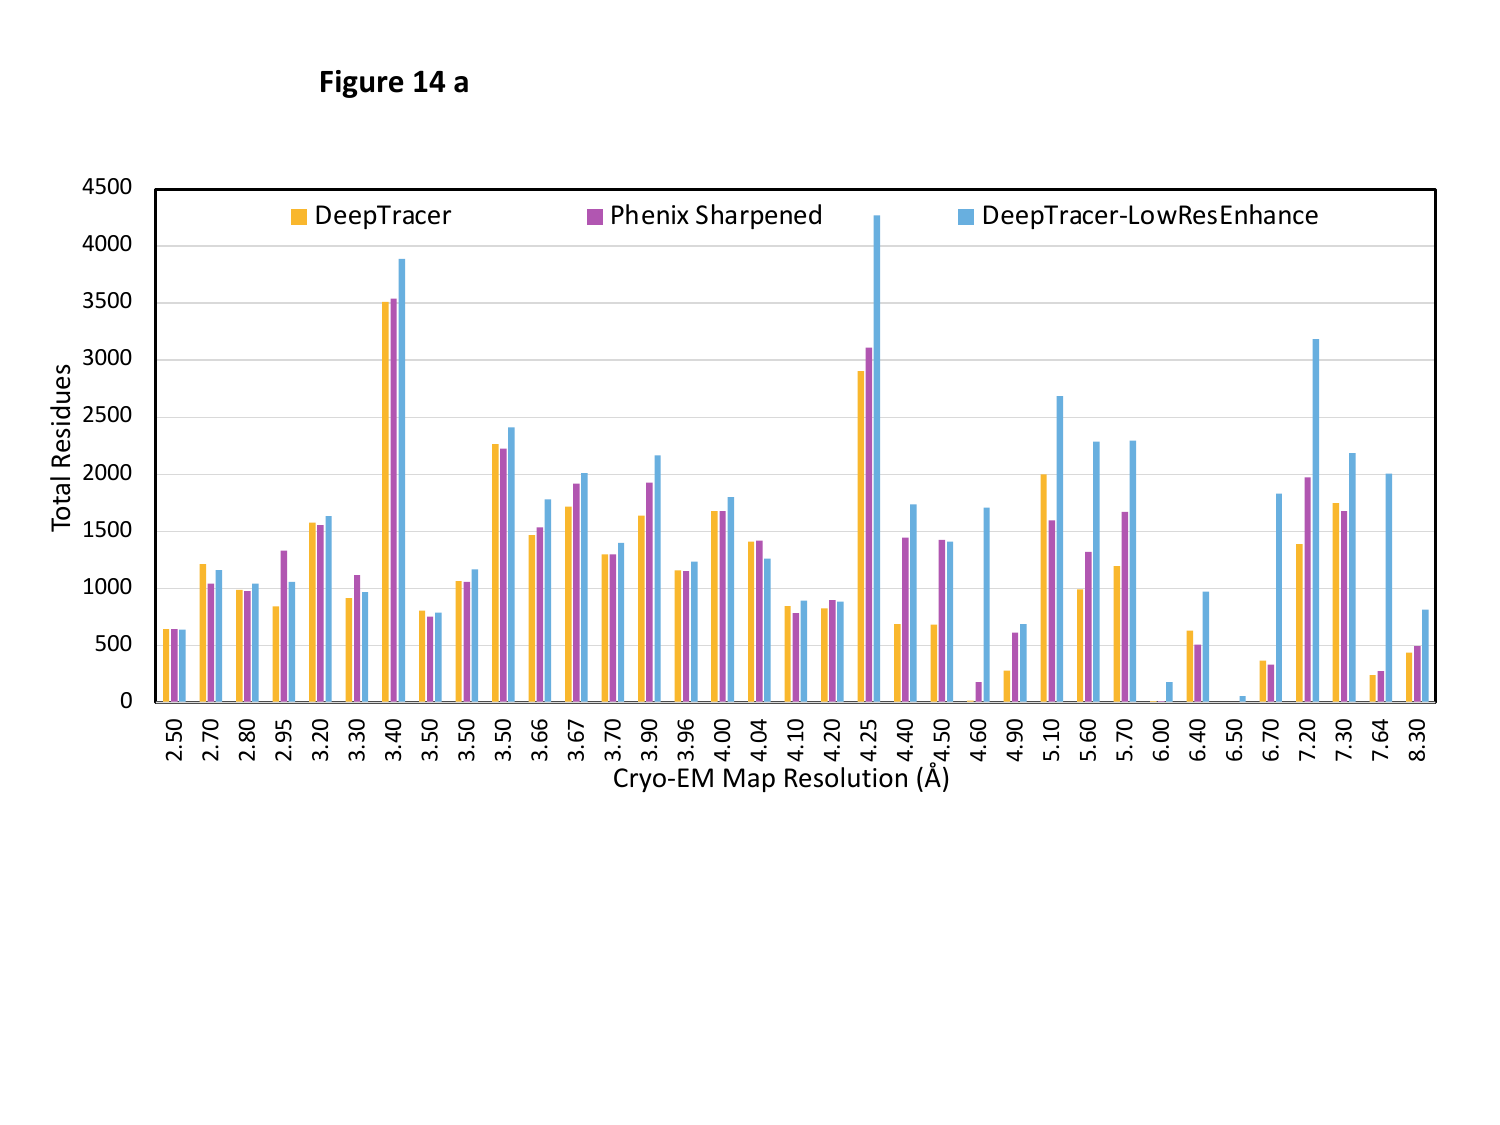}
        \caption{Overall map-model correlation comparison with resolution.}
    \label{fig:appendix-total-residues_a}
    \end{subfigure}%

    \vspace{0.5cm} % Add some vertical space between the subfigures
    
    \begin{subfigure}[t]{0.98\textwidth}
        \centering
        \includegraphics[width=\linewidth]{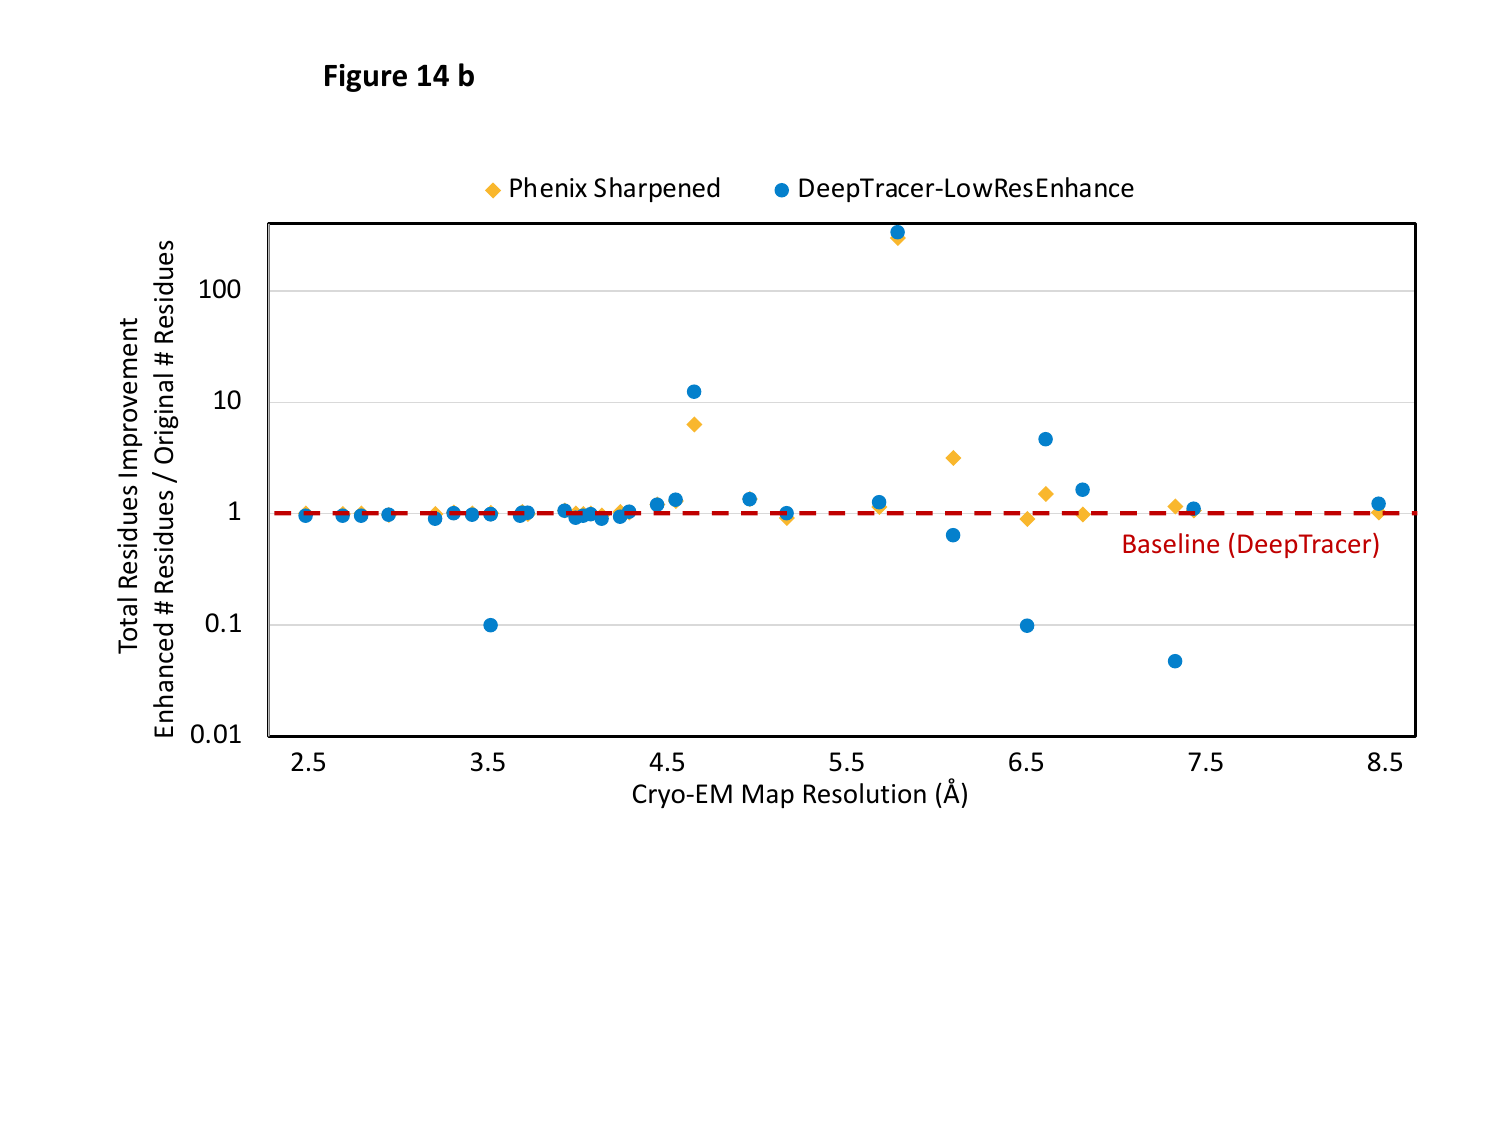}
    \caption{Overall map-model correlation of comparison models with DeepTracer baseline model.}
    \label{fig:appendix-total-residues_b}
    \end{subfigure}
    \caption{Total Residues Comparison between our proposed DeepTracer-LowResEnhance workflow, DeepTracer with Phenix sharpened maps, and original DeepTracer.}
    \label{fig:appendix-total-residues}
\end{figure}

% emd-33798

% ========== Appendix B

% AlphaFold Model

\begin{table}[!htb]
\caption{Summary of AlphaFold Model Results}\label{tab:AF-results}
\begin{tabular*}{\textwidth}{@{\extracolsep{\fill}}p{0.1\textwidth}p{0.15\textwidth}p{0.2\textwidth}p{0.2\textwidth}p{0.2\textwidth}}
\toprule
EMD ID & Stated Resolution & Overall Map-Model Correlation & Total Residues & Residues in Acceptable Density \\
\midrule
        12042 & 2.5 & 0.674 & 717 & 463 \\
        25827 & 2.7 & 0.700 & 1188 & 738 \\
        24219 & 2.8 & 0.532 & 1043 & 733 \\
        23709 & 2.95 & 0.012 & 637 & 295 \\
        0560 & 3.2 & 0.639 & 1594 & 901 \\
        22749 & 3.3 & 0.256 & 424 & 237 \\
        22315 & 3.4 & 0.469 & 4833 & 2720 \\
        11731 & 3.5 & 0.465 & 614 & 308 \\
        13095 & 3.5 & 0.576 & 1158 & 542 \\
        23019 & 3.5 & 0.601 & 2556 & 1469 \\
        11803 & 3.66 & 0.434 & 1762 & 899 \\
        23807 & 3.67 & 0.500 & 2041 & 981 \\
        22776 & 3.7 & 0.374 & 1373 & 793 \\
        22295 & 3.9 & 0.407 & 2022 & 977 \\
        4997 & 3.96 & 0.657 & 1242 & 694 \\
        25801 & 4.0 & 0.433 & 1798 & 999 \\
        23690 & 4.04 & 0.191 & 1390 & 693 \\
        23099 & 4.1 & 0.460 & 888 & 456 \\
        23101 & 4.2 & 0.370 & 887 & 388 \\
        6952 & 4.25 & 0.490 & 4227 & 1635 \\
        23951 & 4.4 & 0.503 & 1739 & 720 \\
        25694 & 4.5 & 0.272 & 1418 & 661 \\
        12637 & 4.6 & 0.322 & 1643 & 715 \\
        24672 & 4.9 & 0.131 & 688 & 163 \\
        33798 & 5.1 & 0.527 & 2691 & 1332 \\
        23929 & 5.6 & 0.449 & 2302 & 808 \\
        3672 & 5.7 & 0.479 & 2460 & 1134 \\
        29072 & 6.0 & 0.111 & 838 & 185 \\
        12602 & 6.4 & 0.420 & 1234 & 435 \\
        26563 & 6.5 & 0.089 & 1356 & 557 \\
        4141 & 6.7 & 0.601 & 1983 & 666 \\
        2183 & 7.2 & 0.062 & 639 & 272 \\
        40758 & 7.3 & 0.660 & 4244 & 1750 \\
        35448 & 7.64 & 0.078 & 1734 & 690 \\
        40320 & 7.75 & No AF model & No AF model & No AF model \\
        17124 & 8.3 & No AF model & No AF model & No AF model \\
        17245 & 8.4 & No AF model & No AF model & No AF model \\
\bottomrule
\end{tabular*}
\end{table}

% DeepTracer Result
\begin{table}[!htb]
\caption{Summary of DeepTracer Model Results}\label{tab:deeptracer-results}
\begin{tabular*}{\textwidth}{@{\extracolsep{\fill}}p{0.1\textwidth}p{0.15\textwidth}p{0.2\textwidth}p{0.2\textwidth}p{0.2\textwidth}}
\toprule
EMD ID & Stated Resolution & Overall Map-Model Correlation & Total Residues & Residues in Acceptable Density \\
\midrule
    12042 & 2.5 & 0.483 & 643 & 495 \\
    25827 & 2.7 & 0.488 & 1214 & 858 \\
    24219 & 2.8 & 0.367 & 987 & 756 \\
    23709 & 2.95 & 0.187 & 842 & 548 \\
    0560 & 3.2 & 0.433 & 1576 & 984 \\
    22749 & 3.3 & 0.280 & 918 & 637 \\
    22315 & 3.4 & 0.519 & 3509 & 2569 \\
    11731 & 3.5 & 0.457 & 806 & 604 \\
    13095 & 3.5 & 0.450 & 1066 & 615 \\
    23019 & 3.5 & 0.427 & 2266 & 1572 \\
    11803 & 3.66 & 0.279 & 1469 & 1071 \\
    23807 & 3.67 & 0.311 & 1719 & 1287 \\
    22776 & 3.7 & 0.277 & 1296 & 1074 \\
    22295 & 3.9 & 0.241 & 1637 & 1348 \\
    4997 & 3.96 & 0.524 & 1156 & 855 \\
    25801 & 4.0 & 0.267 & 1680 & 1309 \\
    23690 & 4.04 & 0.141 & 1411 & 1113 \\
    23099 & 4.1 & 0.306 & 845 & 592 \\
    23101 & 4.2 & 0.229 & 826 & 613 \\
    6952 & 4.25 & 0.353 & 2906 & 1964 \\
    23951 & 4.4 & 0.249 & 687 & 477 \\
    25694 & 4.5 & 0.147 & 684 & 544 \\
    12637 & 4.6 & 0.010 & 17 & 10 \\
    24672 & 4.9 & 0.144 & 280 & 201 \\
    33798 & 5.1 & 0.327 & 2000 & 1412 \\
    23929 & 5.6 & 0.238 & 992 & 804 \\
    3672 & 5.7 & 0.001 & 1196 & 590 \\
    29072 & 6.0 & 0.063 & 12 & 4 \\
    12602 & 6.4 & 0.336 & 629 & 472 \\
    26563 & 6.5 & 0.008 & 6 & 3 \\
    4141 & 6.7 & 0.270 & 369 & 277 \\
    2183 & 7.2 & 0.149 & 1390 & 995 \\
    40758 & 7.3 & 0.479 & 1749 & 1403 \\
    35448 & 7.64 & 0.000 & 239 & 134 \\
    40320 & 7.75 & Failed & Failed & Failed \\
    17124 & 8.3 & 0.175 & 440 & 316 \\
    17245 & 8.4 & Failed & Failed & Failed \\
\bottomrule
\end{tabular*}
\end{table}

% Phenix Sharpened Results
\begin{table}[!htb]
\caption{Summary of \textit{phenix.auto\_sharpen} Model Results} \label{tab:phenix-results}
\begin{tabular*}{\textwidth}{@{\extracolsep{\fill}}p{0.1\textwidth}p{0.15\textwidth}p{0.2\textwidth}p{0.2\textwidth}p{0.2\textwidth}}
\toprule
EMD ID & Stated Resolution & Overall Map-Model Correlation & Total Residues & Residues in Acceptable Density \\
\midrule
    12042 & 2.5 & 0.485 & 644 & 515 \\
    25827 & 2.7 & 0.482 & 1042 & 783 \\
    24219 & 2.8 & 0.367 & 979 & 741 \\
    23709 & 2.95 & 0.181 & 1332 & 757 \\
    0560 & 3.2 & 0.430 & 1556 & 968 \\
    22749 & 3.3 & 0.288 & 1116 & 762 \\
    22315 & 3.4 & 0.521 & 3540 & 2573 \\
    11731 & 3.5 & 0.458 & 752 & 579 \\
    13095 & 3.5 & 0.455 & 1057 & 631 \\
    23019 & 3.5 & 0.429 & 2227 & 1545 \\
    11803 & 3.66 & 0.280 & 1535 & 1130 \\
    23807 & 3.67 & 0.321 & 1920 & 1422 \\
    22776 & 3.7 & 0.275 & 1297 & 1046 \\
    22295 & 3.9 & 0.256 & 1928 & 1537 \\
    4997 & 3.96 & 0.523 & 1152 & 846 \\
    25801 & 4.0 & 0.266 & 1679 & 1308 \\
    23690 & 4.04 & 0.141 & 1420 & 1128 \\
    23099 & 4.1 & 0.295 & 785 & 549 \\
    23101 & 4.2 & 0.236 & 898 & 650 \\
    6952 & 4.25 & 0.362 & 3113 & 2082 \\
    23951 & 4.4 & 0.302 & 1446 & 974 \\
    25694 & 4.5 & 0.190 & 1424 & 1013 \\
    12637 & 4.6 & 0.063 & 180 & 123 \\
    24672 & 4.9 & 0.194 & 615 & 401 \\
    33798 & 5.1 & 0.299 & 1594 & 1114 \\
    23929 & 5.6 & 0.272 & 1319 & 1073 \\
    3672 & 5.7 & 0.299 & 1671 & 1293 \\
    29072 & 6.0 & 0.200 & 12 & 9 \\
    12602 & 6.4 & 0.302 & 507 & 366 \\
    26563 & 6.5 & 0.012 & 6 & 4 \\
    4141 & 6.7 & 0.264 & 334 & 245 \\
    2183 & 7.2 & 0.173 & 1973 & 1430 \\
    40758 & 7.3 & 0.510 & 1680 & 1397 \\
    35448 & 7.64 & 0.000 & 278 & 142 \\
    40320 & 7.75 & 0.020 & 58 & 32 \\
    17124 & 8.3 & 0.180 & 497 & 352 \\
    17245 & 8.4 & 0.038 & 978 & 487 \\
\bottomrule
\end{tabular*}
\end{table}

% DeepTracer-LowResEnhance results
\begin{table}[!htb]
\caption{Summary of DeepTracer-LowResEnhance Results} \label{tab:DTEnhanced-results}
\begin{tabular*}{\textwidth}{@{\extracolsep{\fill}}p{0.1\textwidth}p{0.15\textwidth}p{0.2\textwidth}p{0.2\textwidth}p{0.2\textwidth}}
\toprule
EMD ID & Stated Resolution & Overall Map-Model Correlation & Total Residues & Residues in Acceptable Density \\
\midrule
    12042 & 2.5 & 0.460 & 639 & 471 \\
    25827 & 2.7 & 0.467 & 1161 & 779 \\
    24219 & 2.8 & 0.349 & 1043 & 734 \\
    23709 & 2.95 & 0.182 & 1056 & 605 \\
    0560 & 3.2 & 0.387 & 1634 & 961 \\
    22749 & 3.3 & 0.281 & 969 & 628 \\
    22315 & 3.4 & 0.506 & 3888 & 2532 \\
    11731 & 3.5 & 0.045 & 790 & 285 \\
    13095 & 3.5 & 0.440 & 1165 & 620 \\
    23019 & 3.5 & 0.420 & 2411 & 1589 \\
    11803 & 3.66 & 0.267 & 1780 & 1138 \\
    23807 & 3.67 & 0.314 & 2013 & 1422 \\
    22776 & 3.7 & 0.282 & 1397 & 1045 \\
    22295 & 3.9 & 0.254 & 2166 & 1588 \\
    4997 & 3.96 & 0.478 & 1236 & 790 \\
    25801 & 4.0 & 0.253 & 1803 & 1287 \\
    23690 & 4.04 & 0.138 & 1264 & 1009 \\
    23099 & 4.1 & 0.275 & 892 & 544 \\
    23101 & 4.2 & 0.214 & 886 & 585 \\
    6952 & 4.25 & 0.367 & 4270 & 2603 \\
    23951 & 4.4 & 0.298 & 1734 & 1064 \\
    25694 & 4.5 & 0.194 & 1413 & 1037 \\
    12637 & 4.6 & 0.124 & 1711 & 1006 \\
    24672 & 4.9 & 0.193 & 690 & 407 \\
    33798 & 5.1 & 0.327 & 2687 & 1713 \\
    23929 & 5.6 & 0.299 & 2287 & 1615 \\
    3672 & 5.7 & 0.336 & 2295 & 1732 \\
    29072 & 6.0 & 0.040 & 180 & 30 \\
    12602 & 6.4 & 0.033 & 972 & 299 \\
    26563 & 6.5 & 0.037 & 58 & 31 \\
    4141 & 6.7 & 0.442 & 1832 & 1187 \\
    2183 & 7.2 & 0.007 & 3185 & 1301 \\
    40758 & 7.3 & 0.527 & 2186 & 1780 \\
    35448 & 7.64 & 0.006 & 2006 & 978 \\
    40320 & 7.75 & 0.009 & 202 & 96 \\
    17124 & 8.3 & 0.214 & 817 & 592 \\
    17245 & 8.4 & 0.089 & 1501 & 719 \\
\bottomrule
\end{tabular*}
\end{table}

% Low Res Residues in Acceptable Density Percentage Change
\begin{table}[!htb]
\caption{Comparative Analysis of Percentage Change in Residues within Acceptable Density for Low-Resolution Maps: \textit{phenix.auto\_sharpen} vs. DeepTracer-LowResEnhance (DT-LRE)}\label{tab:low-res-change}
\resizebox{\textwidth}{!}{%
\begin{tabular}{ccccccc}
\toprule
EMD ID & Stated Resolution & DeepTracer Residues & \textit{phenix.auto\_sharpen} Residues & DT-LRE Residues & \textit{phenix} Increase \% & DT-LRE Increase \%\\
\midrule
    25801 & 4.0 & 1309 & 1308 & 1287 & -0.076\% & -1.681\% \\
    23690 & 4.04 & 1113 & 1128 & 1009 & 1.348\% & -9.344\% \\
    23099 & 4.1 & 592 & 549 & 544 & -7.264\% & -8.108\% \\
    23101 & 4.2 & 613 & 650 & 585 & 6.036\% & -4.568\% \\
    6952 & 4.25 & 1964 & 2082 & 2603 & 6.008\% & 32.536\% \\
    23951 & 4.4 & 477 & 974 & 1064 & 104.193\% & 123.061\% \\
    25694 & 4.5 & 544 & 1013 & 1037 & 86.213\% & 90.625\% \\
    12637 & 4.6 & 10 & 123 & 1006 & 1130.000\% & 9960.000\% \\
    24672 & 4.9 & 201 & 401 & 407 & 99.502\% & 102.488\% \\
    33798 & 5.1 & 1412 & 1114 & 1713 & -21.105\% & 21.317\% \\
    23929 & 5.6 & 804 & 1073 & 1615 & 33.458\% & 100.871\% \\
    3672 & 5.7 & 590 & 1293 & 1732 & 119.153\% & 193.559\% \\
    29072 & 6.0 & 4 & 9 & 30 & 125.000\% & 650.000\% \\
    12602 & 6.4 & 472 & 366 & 299 & -22.458\% & -36.653\% \\
    26563 & 6.5 & 3 & 4 & 31 & 33.333\% & 933.333\% \\
    4141 & 6.7 & 277 & 245 & 1187 & -11.552\% & 328.520\% \\
    2183 & 7.2 & 995 & 1430 & 1301 & 43.719\% & 30.754\% \\
    40758 & 7.3 & 1403 & 1397 & 1780 & -0.428\% & 26.871\% \\
    35448 & 7.64 & 134 & 142 & 978 & 5.970\% & 629.851\% \\
    17124 & 8.3 & 316 & 352 & 592 & 11.392\% & 87.342\% \\
    \hline
    \multicolumn{5}{|r|}{Avg} & 87.122\% & 662.539\%  \\ % Average row
\bottomrule
\end{tabular}%
}
\end{table}

% with and without AF
\begin{table}[!htb]
\caption{Evaluating the Impact of AlphaFold Integration on DeepTracer-LowResEnhance (DT-LRE)}\label{tab:with_without_AF}
\small % Adjusts the font size to fit the table within the page width
\begin{tabular}{p{0.08\textwidth}p{0.07\textwidth}p{0.1\textwidth}p{0.1\textwidth}p{0.1\textwidth}p{0.1\textwidth}p{0.1\textwidth}p{0.1\textwidth}}
\toprule
EMD ID & Stated Res. & DT-LRE w/ AF Corr. & DT-LRE w/ AF Res. & DT-LRE w/ AF Acc. Dens. & DT-LRE w/o AF Corr. & DT-LRE w/o AF Res. & DT-LRE w/o AF Acc. Dens. \\
\midrule
    25801 & 4.0   & 0.266 & 1679  & 1308  & 0.268 & 1743  & 1354 \\
    23690 & 4.04  & 0.141 & 1420  & 1128  & 0.137 & 1213  & 977 \\
    23099 & 4.1   & 0.295 & 785   & 549   & 0.311 & 716   & 523 \\
    23101 & 4.2   & 0.236 & 898   & 650   & 0.239 & 870   & 640 \\
    6952  & 4.25  & 0.362 & 3113  & 2082  & 0.357 & 3213  & 2101 \\
    23951 & 4.4   & 0.302 & 1446  & 974   & 0.271 & 780   & 570 \\
    25694 & 4.5   & 0.190 & 1424  & 1013  & 0.179 & 1077  & 851 \\
    12637 & 4.6   & 0.063 & 180   & 123   & 0.013 & 88    & 51 \\
    24672 & 4.9   & 0.194 & 615   & 401   & 0.186 & 450   & 299 \\
    33798 & 5.1   & 0.299 & 1594  & 1114  & 0.345 & 2560  & 1759 \\
    23929 & 5.6   & 0.272 & 1319  & 1073  & 0.285 & 1481  & 1158 \\
    3672  & 5.7   & 0.299 & 1671  & 1293  & 0.314 & 1702  & 1277 \\
    26563 & 6.5   & 0.037 & 58    & 31    & 0.027 & 22    & 16 \\
    4141  & 6.7   & 0.442 & 1832  & 1187  & 0.376 & 866   & 608 \\
    2183  & 7.2   & 0.007 & 3185  & 1301  & 0.008 & 3033  & 1256 \\
    40758 & 7.3   & 0.527 & 2186  & 1780  & 0.523 & 2183  & 1771 \\
    35448 & 7.64  & 0.006 & 2006  & 978   & 0.000 & 1891  & 1048 \\
\bottomrule
\end{tabular}
\end{table}

% Similarity comparison with PDB
\begin{table}[!htb]
\caption{Structure Similarity Comparison Between DeepTracer-LowResEnhance Predictions and Solved Structures for Low-Resolution Maps}\label{tab:similarity_compare}
\begin{tabular}{ccc}
\toprule
EMD ID & Stated Resolution & TM-score \\
\midrule
    25801 & 4.0 & 0.28546 \\
    23690 & 4.04 & 0.19034 \\
    23099 & 4.1 & 0.75046 \\
    23101 & 4.2 & 0.87230 \\
    6952 & 4.25 & 0.71923 \\
    23951 & 4.4 & 0.22524 \\
    25694 & 4.5 & 0.75322 \\
    12637 & 4.6 & 0.39101 \\
    24672 & 4.9 & 0.54801 \\
    33798 & 5.1 & 0.43477 \\
    23929 & 5.6 & 0.23485 \\
    3672 & 5.7 & 0.13707 \\
    29072 & 6.0 & 0.04932 \\
    12602 & 6.4 & 0.11079 \\
    26563 & 6.5 & 0.01888 \\
    4141 & 6.7 & 0.30552 \\
    2183 & 7.2 & 0.20278 \\
    40758 & 7.3 & 0.06805 \\
    35448 & 7.64 & 0.34861 \\
\bottomrule
\end{tabular}
\end{table}

% Resolution improvements DeepTracer-LowResEnhance
\begin{table}[!htb]
\caption{Enhanced Cryo-EM Map Resolution via DeepTracer-LowResEnhance}\label{tab:res-improvements}
\small % Adjusts the font size to fit the table within the page width
\begin{tabular}{ccc}
\toprule
EMD ID & Stated Res. & DT-LRE Enhanced Res. \\
\midrule
    12042 & 2.5 & 1.86 \\
    25827 & 2.7 & 1.88 \\
    24219 & 2.8 & 1.91 \\
    23709 & 2.95 & 2.05 \\
    0560 & 3.2 & 1.95 \\
    22749 & 3.3 & 2.13 \\
    22315 & 3.4 & 2.00 \\
    11731 & 3.5 & 2.31 \\
    13095 & 3.5 & 2.24 \\
    23019 & 3.5 & 2.13 \\
    11803 & 3.66 & 2.16 \\
    23807 & 3.67 & 2.02 \\
    22776 & 3.7 & 2.32 \\
    22295 & 3.9 & 2.40 \\
    4997 & 3.96 & 2.09 \\
    25801 & 4.0 & 2.06 \\
    23690 & 4.04 & 2.96 \\
    23099 & 4.1 & 2.05 \\
    23101 & 4.2 & 2.07 \\
    6952 & 4.25 & 2.26 \\
    23951 & 4.4 & 3.44 \\
    25694 & 4.5 & 2.87 \\
    12637 & 4.6 & 2.18 \\
    24672 & 4.9 & 2.92 \\
    33798 & 5.1 & 2.48 \\
    23929 & 5.6 & 4.16 \\
    3672 & 5.7 & 3.38 \\
    29072 & 6.0 & 2.99 \\
    12602 & 6.4 & 3.47 \\
    26563 & 6.5 & 6.23 \\
    4141 & 6.7 & 4.05 \\
    2183 & 7.2 & 5.4 \\
    40758 & 7.3 & 3.32 \\
    35448 & 7.64 & 3.86 \\
    40320 & 7.75 & 7.05 \\
    17124 & 8.3 & 5.93 \\
    17245 & 8.4 & 8.01 \\
\bottomrule
\end{tabular}
\end{table}
